# Supplementary material for: HGDiffuser: Efficient Task-Oriented Grasp Generation via Human-Guided Grasp Diffusion Models
Source: arXiv:2503.00508 source file (2025-03-01)
Supplement: Supplementary file 1 [file appendix.tex]

\onecolumn

\begin{appendices}

\section{}

\subsection{Language Augmented TaskGrasp (LA-TaskGrasp) Dataset}

This section presents the natural language prompts utilized to generate object class and task descriptions within the LA-TaskGrasp dataset. Additionally, we provide detailed examples of object class descriptions (\textit{``Mug"}, \textit{``Spoon"}, and \textit{``Hammer"}) and task descriptions (\textit{``Sweep"}, \textit{``Screw"}, and \textit{``Slice"}). Following that, we present a list of 53 language instruction templates, consisting of 11 templates derived from previous work and 42 templates generated through LLM data augmentation. Lastly, we offer 18 LA-TaskGrasp dataset examples, each of which includes 6 DoF task-oriented grasp poses, a language instruction, an object class description paragraph, and a task description paragraph.\\

\subsubsection{Object Class Description Prompts} 

\begin{itemize}
    \setlength{\itemsep}{5pt}
    \item ``\textit{Describe the shape/geometry of household object [obj] in a detailed and scientific response:}"
    \item ``\textit{Describe the common use/function of household object [obj] in a detailed and scientific response:}"
    \item ``\textit{Describe what household objects have similar shapes/geometries to [obj] in a detailed and scientific response:}"
    \item ``\textit{Describe what household objects have similar uses/functions to [obj] in a detailed and scientific response:}" \\
\end{itemize} 

\subsubsection{Object Class Description Examples}\

\begin{table}[h]
\centering

\setlength\tabcolsep{5pt}%调列距
\begin{tabular}{lcc}
\hline
\multicolumn{1}{c}{\textbf{Class}}                  & \textbf{Property Description}                                                                                                                                                                                                                                                                                                                             & \textbf{Similarity Description}                                                                                                                                                                                                                                                                                                                     \\ \hline \specialrule{0em}{3pt}{3pt}
\multirow{6}{*}{\textit{Mug}}                       & \begin{tabular}[c]{@{}c@{}}(shape)\textit{``The mug is cylindrical in shape, with a slightly rounded} \\ \textit{base leading  up to straight walls which eventually taper} \\ \textit{slightly towards the rim."}\end{tabular}                                                                                                                                             & \begin{tabular}[c]{@{}c@{}}(similar shape)\textit{``Mugs typically have a cylindrical shape with a} \\ \textit{slightly tapered top and a curved handle; objects with similar} \\ \textit{shapes include bottles and vases."}\end{tabular}                                                                                                                             \\ \specialrule{0em}{3pt}{3pt}
                                           & \begin{tabular}[c]{@{}c@{}}(use)\textit{``A mug is a cylindrical drinking vessel typically used to} \\ \textit{hold  hot beverages such as coffee, tea, hot chocolate,} \\ \textit{or soup. The curved shape of the mug allows liquids} \\ \textit{to be held and consumed while reducing splashes} \\ \textit{and spills."}\end{tabular}                                                      & \begin{tabular}[c]{@{}c@{}}(similar use)\textit{``Mugs and other household objects, such as glasses,} \\ \textit{jars, and other containers, can all be used to hold and contain} \\ \textit{liquids, such as hot or cold drinks. In addition, certain mugs,} \\ \textit{such as those with handles, can also be used to stir and mix} \\ \textit{drinks and other items."}\end{tabular} \\ \specialrule{0em}{3pt}{3pt} \hline \specialrule{0em}{3pt}{3pt}
\multirow{5}{*}{\textit{Spoon}}                     & \begin{tabular}[c]{@{}c@{}}(shape)\textit{``The spoon has a slightly curved bowl shape with a} \\ \textit{long, narrow handle extending diagonally from the bowl in} \\ \textit{the opposite direction to the spoon’s curved edge."}\end{tabular}                                                                                                                            & \begin{tabular}[c]{@{}c@{}}(similar shape)\textit{``A teaspoon and a spoon have a similar shape,} \\ \textit{with both utensils curved at the bowl with a long, thin handle.} \\ \textit{In addition, a soup spoon has a shape similar to a spoon."}\end{tabular}                                                                                                      \\ \specialrule{0em}{3pt}{3pt}
                                           & \begin{tabular}[c]{@{}c@{}}(use)\textit{``A spoon is a unit of measurement for dry and liquid} \\ \textit{ingredients that equals approximately three teaspoons,} \\ \textit{and is used for serving, measuring, and mixing foods."}\end{tabular}                                                                                                                            & \begin{tabular}[c]{@{}c@{}}(similar function)\textit{``A spoon is a utensil commonly used for} \\ \textit{measuring, stirring, and serving food. Household objects} \\ \textit{similar in function include a measuring cup, and soup ladle."}\end{tabular}                                                                                                             \\ \specialrule{0em}{3pt}{3pt} \hline \specialrule{0em}{3pt}{3pt}
\multirow{7}{*}{\textit{Hammer}}                    & \begin{tabular}[c]{@{}c@{}}(shape)\textit{``The hammer has an elongated cylindrical shape with a} \\ \textit{flattened striking face at oneend and a handle at the other end."}\end{tabular}                                                                                                                                                                        & \begin{tabular}[c]{@{}c@{}}(similar shape)\textit{``A hammer has a similar shape as a meat} \\ \textit{tenderizer, an ice pick, and a nail puller."}\end{tabular}                                                                                                                                                                                             \\ \specialrule{0em}{3pt}{3pt}
                                           & \begin{tabular}[c]{@{}c@{}}(use)\textit{``The hammer is a tool used to deliver an impulse force to an} \\ \textit{object. It works by transferring kinetic energy from the handle} \\ \textit{to the striking head of the hammer, allowing the user to drive} \\ \textit{nails, shape and flatten objects, and otherwise manipulate} \\ \textit{the material being worked upon."}\end{tabular} & \begin{tabular}[c]{@{}c@{}}(similar functions)\textit{``A household object that serves a similar} \\ \textit{function to that of a hammer is a kitchen mallet, which is} \\ \textit{used to pound, tenderize, and flatten food. Another} \\ \textit{common household item that serves a similar} \\ \textit{purpose is a rubber mallet.}\end{tabular}                                    \\  \specialrule{0em}{3pt}{3pt}  \hline
\end{tabular}
\caption{Examples of object class descriptions}
\end{table}

\newpage

\subsubsection{Task Description Prompts}
\begin{itemize}
    \setlength{\itemsep}{5pt}
    \item ``\textit{Describe what household objects can be used to [task] in a detailed and scientific response:}"
    \item ``\textit{Describe what household objects support the function of [task] in a detailed and scientific response:}"
    \item ``\textit{Describe what verbs are semantically close to [task] in a detailed and scientific response:}"
    \item ``\textit{Describe what verbs achieve similar effects to ’[task] an object’ in a detailed and scientific response:}" \\
\end{itemize} 

\subsubsection{Task Description Examples}\

\begin{table}[h]
\centering

\setlength\tabcolsep{5pt}%调列距
\begin{tabular}{lcc}
\hline
\multicolumn{1}{c}{\textbf{Task}}                   & \textbf{Affordance Description}                                                                                                                                                                                                                                                                                                                           & \textbf{Relevance Description}                                                                                                                                                                                                                                                                                                                      \\ \hline \specialrule{0em}{3pt}{3pt}
\multicolumn{1}{c}{\multirow{5}{*}{\textit{Sweep}}} & \begin{tabular}[c]{@{}c@{}}(use)\textit{``Household objects that can be used to sweep include brooms,} \\ \textit{dustpans and mops.} "\end{tabular}                                                                                                                                                                                                                & \begin{tabular}[c]{@{}c@{}}(closeness)\textit{``Verbs that are semantically close to sweep} \\ \textit{include cleanse, purify, and eradicate."}\end{tabular}                                                                                                                                                                                                 \\  \specialrule{0em}{3pt}{3pt}
\multicolumn{1}{c}{}                       & \begin{tabular}[c]{@{}c@{}}(function)\textit{``Household objects such as a broom, dustpan, and mop help} \\ \textit{to support the sweeping function by providing a tool with which to} \\ \textit{sweep away dust and debris. The broom helps to physically remove} \\ \textit{dirt and dust from the floors and other surfaces."}\end{tabular}                                      & \begin{tabular}[c]{@{}c@{}}(similar effect)\textit{``The action of sweeping an object can be} \\ \textit{described as a type of displacement, in which the object is} \\ \textit{moved across a surface in a steady, sweeping motion. This} \\ \textit{is similar to actions like pushing, dragging, and gliding."}\end{tabular}                                                \\  \specialrule{0em}{3pt}{3pt} \hline  \specialrule{0em}{3pt}{3pt}
\multirow{6}{*}{\textit{Screw}}                     & \begin{tabular}[c]{@{}c@{}}(use)\textit{``Household objects that can be used to screw in objects} \\ \textit{include screwdrivers, managed screwdrivers, and various tools} \\ \textit{with rotating handles, such as adjustable wrenches, pliers,} \\ \textit{and socket wrenches."}\end{tabular}                                                                                    & \begin{tabular}[c]{@{}c@{}}(closeness)\textit{``Verbs that are semantically close to ‘screw’} \\ \textit{might include ‘twist’, ‘fasten’, or ‘tighten’, as these all} \\ \textit{fall within the general semantic domain of attaching or} \\ \textit{fastening objects or components together."}\end{tabular}                                                                   \\  \specialrule{0em}{3pt}{3pt}
                                           & \begin{tabular}[c]{@{}c@{}}(function)\textit{``Household objects such as screwdrivers and} \\ \textit{power drills provide the necessary torque required to} \\ \textit{turn a screw and hold it in place, providing support} \\ \textit{for the function of the screw."}\end{tabular}                                                                                                & \begin{tabular}[c]{@{}c@{}}(similar effect)\textit{``Verbs such as ’fasten’, ’attach’, and ’secure’} \\ \textit{can have similar effects to ’screw an object’, by joining} \\ \textit{two pieces of material together and providing} \\ \textit{a strong connection."}\end{tabular}                                                                                             \\  \specialrule{0em}{3pt}{3pt} \hline  \specialrule{0em}{3pt}{3pt}
\multirow{5}{*}{\textit{Slice}}                     & \begin{tabular}[c]{@{}c@{}}(use)\textit{``Household objects that can be used to slice include knives,} \\ \textit{graters, mandolines, and vegetable peelers. These objects} \\ \textit{typically have blades that are designed to cut through a} \\ \textit{variety of food items."}\end{tabular}                                                                                    & \begin{tabular}[c]{@{}c@{}}(closeness)\textit{``Verbs semantically close to slice include} \\ \textit{chop, divide, section, mince, dice and shred, as} \\ \textit{they all involve cutting an object into smaller pieces,} \\ \textit{either directly or through an intermediary tool."}\end{tabular}                                                                          \\  \specialrule{0em}{3pt}{3pt}
                                           & \begin{tabular}[c]{@{}c@{}}(function)\textit{``Household objects that support the function of} \\ \textit{slicing include knives with sharp edges and fine serrations,} \\ \textit{as well as manual slicers that use an adjustable blade} \\ \textit{to create uniform slices."}\end{tabular}                                                                                        & \begin{tabular}[c]{@{}c@{}}(similar effect)\textit{``Verbs such as cleave, cut, and divide} \\ \textit{can also achieve the same effect as slicing an object,} \\ \textit{by physically splitting the object into two} \\ \textit{or more distinct parts."}\end{tabular}                                                                                                        \\  \specialrule{0em}{3pt}{3pt} \hline
\end{tabular}
\caption{Examples of task descriptions}
\end{table}

\newpage

\subsubsection{Language Instruction Templates}\

\begin{table}[h]
\centering

\begin{tabular}{cc}
\hline
\multicolumn{2}{c}{\textbf{Language Instruction Templates}}                                                                                                                                                                       \\ \hline
\textit{``use the \textless{}obj\textgreater to \textless{}task\textgreater{}"}                                   & \textit{``use the \textless{}obj\textgreater to perform \textless{}tasking\textgreater{}"}                            \\
\textit{``\textless{}task\textgreater things with the \textless{}obj\textgreater{}"}                                & \textit{``use the \textless{}obj\textgreater to \textless{}task\textgreater something"}                               \\
\textit{``executing \textless{}tasking\textgreater with the \textless{}obj\textgreater{}"}                          & \textit{``use the \textless{}obj\textgreater to conduct \textless{}tasking\textgreater{}"}                            \\
\textit{``utilize the \textless{}obj\textgreater to \textless{}task\textgreater{}"}                                 & \textit{``just use the \textless{}obj\textgreater to \textless{}task\textgreater{}"}                                  \\
\textit{``using a \textless{}obj\textgreater to \textless{}task\textgreater{}"}                                     &\textit{``do \textless{}tasking\textgreater with the \textless{}obj\textgreater{}"}                                   \\
\textit{``perform \textless{}tasking\textgreater with the \textless{}obj\textgreater{}"}                            & \textit{``perform \textless{}tasking\textgreater using the \textless{}obj\textgreater{}"}                             \\
\textit{``bring the \textless{}obj\textgreater out to \textless{}task\textgreater{}"}                               & \textit{``to \textless{}task\textgreater{}, get the \textless{}obj\textgreater{}" }                                   \\
\textit{``find the \textless{}obj\textgreater so that you can \textless{}task\textgreater{}"}                       & \textit{``get the \textless{}obj\textgreater and start \textless{}tasking\textgreater{}"},                            \\
\textit{``bring out the \textless{}obj\textgreater to \textless{}task\textgreater{}"}                               & \textit{``perform \textless{}tasking\textgreater with the \textless{}obj\textgreater{}"}                              \\
\textit{``using a \textless{}obj\textgreater to do \textless{}tasking\textgreater{}"}                               & \textit{``make use of the \textless{}obj\textgreater to \textless{}task\textgreater{}"}                               \\
\textit{``grab the \textless{}obj\textgreater to \textless{}task\textgreater{}"}                                    & \textit{``pick up the \textless{}obj\textgreater to \textless{}task\textgreater{}"}                                   \\
\textit{``to \textless{}task\textgreater{}, hold the \textless{}obj\textgreater in your hand"}                      & \textit{``hold the \textless{}obj\textgreater in your hand and \textless{}task\textgreater{}" }                       \\
\textit{``in order to \textless{}task\textgreater{}, grasp the \textless{}obj\textgreater{}"}                       & \textit{``grasp the \textless{}obj\textgreater in order to \textless{}task\textgreater{}"}                            \\
\textit{``if you want to \textless{}task\textgreater{}, hold the \textless{}obj\textgreater{}"}                     & \textit{``grip the \textless{}obj\textgreater to \textless{}task\textgreater{}"}                                      \\
\textit{``\textless{}task\textgreater with the \textless{}obj\textgreater{}"}                                       & \textit{``grasp the \textless{}obj\textgreater in a way that allows for \textless{}tasking\textgreater{}"}            \\
\textit{``holding the \textless{}obj\textgreater in a \textless{}tasking\textgreater{}-friendly manner"}            & \textit{``take a \textless{}tasking\textgreater{}-friendly hold of the \textless{}obj\textgreater{}" }                \\
\textit{``make sure you have a \textless{}tasking\textgreater{}-friendly grip on the \textless{}obj\textgreater{}"} & \textit{``hold the \textless{}obj\textgreater in a \textless{}tasking\textgreater manner"}                            \\
\textit{``grip the \textless{}obj\textgreater in a \textless{}tasking\textgreater{}-friendly manner"}               & \textit{``ensure you have a \textless{}tasking\textgreater{}-friendly grip on the \textless{}obj\textgreater{}"}      \\
\textit{``use the \textless{}obj\textgreater to \textless{}task\textgreater things"}                                & \textit{``performing \textless{}tasking\textgreater with the \textless{}obj\textgreater{}"}                           \\
\textit{``use the \textless{}obj\textgreater to accomplish \textless{}tasking\textgreater{}"}                       & \textit{``\textless{}tasking\textgreater with the \textless{}obj\textgreater{}"}                                      \\
\textit{``do \textless{}tasking\textgreater using the \textless{}obj\textgreater{}"}                                & \textit{``fetch the \textless{}obj\textgreater to \textless{}task\textgreater{}"}                                     \\
\textit{``find the \textless{}obj\textgreater and then \textless{}task\textgreater{}"}                              & \textit{``obtain the \textless{}obj\textgreater for \textless{}tasking\textgreater{}"}                                \\
\textit{``use the \textless{}obj\textgreater to conduct \textless{}tasking\textgreater{}"}                          & \textit{``grasp the \textless{}obj\textgreater to \textless{}task\textgreater{}"}                                     \\
\textit{``taking hold of the \textless{}obj\textgreater{}, \textless{}task\textgreater{}"}                          & \textit{``to \textless{}task\textgreater{}, grasp the \textless{}obj\textgreater{}"}                                  \\
\textit{``to \textless{}task\textgreater{}, take hold of the \textless{}obj\textgreater{}"}                         & \textit{``get the \textless{}obj\textgreater to \textless{}task\textgreater{}"}                                       \\
\textit{``grasp the \textless{}obj\textgreater in a way that allows you to \textless{}task\textgreater{}"}          & \textit{``ensure you grasp the \textless{}obj\textgreater in a way that allows for \textless{}tasking\textgreater{}"} \\
\textit{``hold the \textless{}obj\textgreater in a \textless{}tasking\textgreater position"}                        &                                                                                                             \\ \hline
\end{tabular}
\caption{Language instruction templates}
\end{table}

\newpage

\subsubsection{Dataset Examples} \

\begin{figure}[h]
  \centering
  % \vspace*{-0.2in}
  \begin{tikzpicture}[inner sep = 0pt, outer sep = 0pt]
    \node[anchor=south west] (fnC) at (0in,0in)
      {\includegraphics[height=6.8in,clip=true,trim=0in 0in 0in 0in]{image/la-taskgrasp_example/la-taskgrasp_examples_all.jpg}};
  \end{tikzpicture}
    % \vspace*{-0.1in}
  \caption{Dataset examples, each of which includes 6 DoF task-oriented grasp poses, a language instruction, an object class description paragraph, and a task description paragraph. Here, we only show part of the paragraphs. All the grasp poses are colored by their task compatibility scores (green is higher).} 
  % \label{fig:concept}
  % \vspace*{-0.3in}
\end{figure}

\newpage

\subsection{Additional Experimental Setup}
This section aims to provide further information regarding the experimental setup employed for both perception and real-robot experiments. \\

\subsubsection{Training Hyper-Parameters} \

\begin{table}[h]

\centering
\begin{tabular}{lc}
\hline
\multicolumn{2}{l}{\textbf{Basic Setting}}                      \\ \hline
Batch Size           & 32                              \\
\# of Points         & 4096                            \\
\# of Epochs         & 50                              \\ \hline
\multicolumn{2}{l}{\textbf{Optimization Setting}}               \\ \hline
Optimizer            & Adam                            \\
Learning Rate                  & 0.0001                          \\
Learning Rate Decay             & 0.7                             \\
Decay Step           & 2e4                             \\
Weight Decay         & 0.0001                          \\
Learning Rate Clip              & 1e-5                            \\ \hline
\multicolumn{2}{l}{\textbf{PointNet++ Setting}}                 \\ \hline
\# of SA Layers      & 3                               \\
\# of Sampled Points & 512, 128, 1                     \\
Embedding Sizes      & 320, 640, 1024                  \\ \hline
\multicolumn{2}{l}{\textbf{Data Preprocessing}}                 \\ \hline
Scaling              & True                            \\
Mean Centering       & True                            \\
Random Rotation      & True                            \\
Random Jitter        & True                            \\
Random Dropout       & True                            \\ \hline
\multicolumn{2}{l}{\textbf{Hardware Resource}}                  \\ \hline
CPU                  & 12th Gen Intel® Core™ i9-12900K \\
\# of  CPU Cores     & 24                              \\
GPU                  & Nvidia RTX 3090                 \\ \hline
\multicolumn{2}{l}{\textbf{LLM Setting}}                  \\ \hline
Model              & OpenAI GPT-3     \\
Engine             & \textit{text-davinci-003} \\
Prompt Type             & text             \\
Temperature        & 1.0              \\
Max Tokens        & 256              \\
Top P             & 1.0              \\
Frequency Penalty & 0.0              \\
Presence Penalty  & 0.0              \\ \hline
\end{tabular}
\caption{Training hyper-parameter setting}
\end{table}

\newpage

\subsubsection{Real-Robot Experiment} \ 

\begin{figure}[th]
  \centering
  \vspace*{-0.2in}
  \begin{tikzpicture}[inner sep = 0pt, outer sep = 0pt]
    \node[anchor=south west] (fnC) at (0in,0in)
      {\includegraphics[height=1.5in,clip=true,trim=0in 0in 0in 0in]{image/supp/real-robot-setup-no-bg.jpg}};
  \end{tikzpicture}
    % \vspace*{-0.1in}
  \caption{Real-robot experimental setup: a Kinova Gen3 robotic arm with a Robotiq parallel jaw gripper (left) and an Intel RealSense D435 RGB camera (right) with eye-in-hand calibration.}
  % \label{fig:real-robot}
  % \vspace*{-0.3in}
\end{figure}

\begin{figure}[h]
  \centering
  \vspace*{-0.1in}
  \begin{tikzpicture}[inner sep = 0pt, outer sep = 0pt]
    \node[anchor=south west] (fnC) at (0in,0in)
      {\includegraphics[height=2.2in,clip=true,trim=0in 0in 0in 0in]{image/supp/test_objects.jpeg}};
  \end{tikzpicture}
    % \vspace*{-0.3in}
  \caption{Test objects collected from our laboratory and YCB dataset.}
  % \label{fig:real-robot}
  % \vspace*{-0.3in}
\end{figure}

\begin{figure}[h]
  \centering
  \vspace*{-0.2in}
  \begin{tikzpicture}[inner sep = 0pt, outer sep = 0pt]
    \node[anchor=south west] (fnC) at (0in,0in)
      {\includegraphics[height=2.5in,clip=true,trim=0in 0in 0in 0in]{image/supp/real-robot-pipeline+.png}};
  \end{tikzpicture}
    % \vspace*{-0.3in}
  \caption{Pipeline of real-robot experiment with intermediate results.}
  % \label{fig:real-robot}
  % \vspace*{-0.3in}
\end{figure}

\newpage

% \subsection{Additional Results}

% \subsubsection{Task-Oriented Grasping Experiments} \ 

% \subsubsection{Task-Oriented Manipulation Experiments} \ 

% \newpage

\subsection{Discussion}
In this section, we discuss the limitations of GraspGPT. Potential solutions are also provided as part of our future work.
\begin{itemize}
    \setlength{\itemsep}{5pt}
    \item \textbf{LLM Knowledge Filtering and Selection}  

    As previously mentioned, we do not process the language data returned by an LLM, which can result in language descriptions containing imprecise or false commonsense knowledge. We identify two typical errors in the generated language descriptions: (1) Part-of-speech error. Since certain words have multiple uses as nouns and verbs, LLM occasionally returns object class knowledge even when prompted with task description prompts, or vice versa. For instance, when we prompt the LLM for the task description of verb \textit{``ladle"} (e.g., \textit{``Describe what household objects support the function of `ladle' in a detailed and scientific response:"}), the LLM might respond with \textit{``A ladle is a utensil that is typically long-handled, with a deep dish or scoop at the end. It is usually made of metal or plastic and is used to serve or measure hot liquids such as soup, sauce, or gravy."} (2) Mismatching descriptions. Due to significant intra-class variances, the LLM-generated object class descriptions may not precisely match the properties of actual object instances. For example, the object class description of \textit{``frying pan"} could be:  \textit{``The geometry of a frying pan is generally cylindrical, with sloping sides and a flat base to evenly disperse heat while cooking."} However, the actual object instance might be square-shaped. To address the first error, GraspGPT should be able to inspect the semantic meaning of the generated language description and verify if it meets the prompt's intention. To tackle the second error, a potential solution would involve incorporating a multi-modal model, such as \href{https://arxiv.org/abs/2301.12597}{BLIP-2}, which can generate language descriptions based on the visual content provided. This integration would require GraspGPT to process additional visual inputs, such as RGB images.
        
    \item \textbf{Task-Oriented Pick and Place} 
    
    Our current work focuses on addressing the challenge of task-oriented grasping/picking. However, to achieve successful tool manipulation, the robot must also anticipate the subsequent motion of the tool and effectively interact with the target object. For instance, when inserting a nail into a slot, the robot needs to perform the following steps: (1) securely grasp the hammer by its handle, (2) guide the hammer towards the nail, assuming the nail is initially positioned halfway inside the slot, and (3) forcefully pound the nail into the slot. While GraspGPT has progressed in addressing the initial task-oriented grasping step, the subsequent steps are currently simplified with pre-defined motion primitives. Recent works, such as \href{https://arxiv.org/abs/2112.05124}{Neural Descriptor Fields}, approach tool manipulation as a pick-and-place task. This involves predicting the grasp point on the tool object (i.e., task-oriented picking) and determining the effect point on the target object (i.e., task-oriented placing). Since we currently use rule-based heuristics to determine the effect point, the robot cannot model the relative pose between the tool object and the target object. Ideally, the robot should adjust the effect point depending on the grasp point. A failure case can be found in the supplementary video. We plan to expand the capabilities of GraspGPT from task-oriented grasping to task-oriented pick and place, leveraging both grasping and placement knowledge from an LLM.
        
    \item \textbf{Single-Stage Architecture} 
    
    GraspGPT currently follows a two-stage, sample-and-evaluate approach, similar to previous works. While this design choice simplifies the complexity of constructing GraspGPT, it introduces a reliance on a pre-trained task-agnostic grasp sampler. As the grasp sampler solely considers geometry information without incorporating semantic priors about the tool to be grasped, it uniformly samples over the given point cloud. However, during robot interaction, only specific functional/affordance regions of a tool are engaged, while non-functional regions remain untouched. This uniform sampling approach makes GraspGPT inefficient for real-time inference. Moreover, GraspGPT assumes all the candidate grasp poses generated by the grasp sampler are stable. However, the sampler may output marginal/unstable grasp poses, which are susceptible to perturbances such as unpredicted contact or calibration error. An example can be found in the supplementary video. Future research aims to integrate task-agnostic sampling and task-oriented evaluation within an end-to-end architecture, enabling the direct prediction of task-oriented grasp poses from given point clouds. This approach is anticipated to consider both stability and task compatibility simultaneously. 
    
    \item \textbf{Simultaneous Affordance Learning} 
    
     A closely related task to task-oriented grasping is affordance recognition, where the robot identifies specific regions on an object for various types of interactions. Previous studies, such as the \href{https://ieeexplore.ieee.org/abstract/document/9364360}{Affordance Keypoint Detection Network} (\textit{AffKP}), have demonstrated the benefits of joint learning of affordance segmentation for task-oriented grasping and manipulation. In future work, we aim to incorporate affordance learning into the GraspGPT framework. We anticipate that simultaneously learning these two objectives would mutually enhance their performance. On the one hand, affordance learning would assist the robot in identifying the relevant regions to grasp for a given task. On the other hand, the supervision provided by task-oriented grasping could serve as weak supervision for affordance recognition. Equipping the robot with affordance recognition capability also opens up possibilities for other tasks, such as task-driven object retrieval/selection and semantic scene understanding.

\end{itemize}

\end{appendices}
